# Supplementary material for: Robust Agility via Learned Zero Dynamics Policies
Source: arXiv:2409.06125 source file (2024-09-10)
Supplement: Supplementary file 1 [file AppendixII.tex]

\section{Appendix II}

Continuous time:

State: $\mathbf{x}, \mathbf{x}^+, \mathbf{x}^-$

Input: $\mathbf{u}$

Actuated: $\boldsymbol{\eta}$

Unactuated: $\mathbf{z}$

Policy: $\boldsymbol \psi_{\b\theta}$

Output: $\mathbf{y}$

Error: $\mathbf{e}$
\\

Discrete time:

State: $\mathbf{x}_k, \mathbf{x}_k^+, \mathbf{x}_k^-$

Input: $\mathbf{v}_k$

Optimal Input: $\mathbf{v}_k^*$

Actuated: $\boldsymbol{\eta}_k$

Unactuated: $\mathbf{z}_k$

Actuated on the manifold: $\boldsymbol \eta^{\mathcal{Z}}_k = \b\psi_{\b \theta}(\b z_k)$

Post impact actuated on manifold: $(\boldsymbol \eta^{\mathcal{Z}}_k)^+$
\\

The surface: $\mathcal{Z}$

System under impulsive effect: $\mathscr{H}$

Parameter set: $P$

Constrained Parameter set: $\mathcal{V}(\mathbf x)\subset P$

Diffeo: $\boldsymbol \Phi$

List of reserved symbols: $\mathbf{D}, \mathbf{C}, \mathbf{B}, \mathbf{H}, \mathbf{f}, \mathbf{g}, \boldsymbol \Delta, \mathbf{F}, \boldsymbol{\Omega}$

\subsection{Deriving the discrete time dynamics}

To begin, let the state of the robot be described by $\b q = (\b p, q, \b \theta, \ell)\in\mathcal{Q}$ where $\b p\in\R^3$ represents the global position in world frame, $q\in \mathbb{S}^3$ the robot's orientation quaternion, $\b \theta_i\in \mathbb{S}^1$ the flywheel angle of the $i^{th}$ motor and $\ell\in\R$ the foot position. Taking the velocities to be $\b v = (\dot{\b p}, \b\omega, \dot{\b \theta}, \dot\ell) \in T_\b q\mathcal{Q}$ for $\b \omega \in \mathfrak{s}^3$ the body frame angular rates, we can represent the full state as $\b x = (\b q, \b v)\in \mathcal{X}\triangleq T\mathcal{Q}$. 

Hopping robots have two distinct dynamic modes -- the flight phase $f$ when they are in the air and the ground phase $g$ when they are in contact with the ground. Letting $p_z:\mathcal{Q}\to\R$ return the height of the foot and $\ell_0\in\R$ represent the nominal spring length, these domains are defined by $\mathcal{D}_f\triangleq\{\b x~|~ p_z(\b q) > 0\}\subset\mathcal{X}$ and $\mathcal{D}_g = \{ \b x~|~ \ell < \ell_0\}\subset\mathcal{X}$. In these continuous domains, the dynamics are governed by the Euler Lagrange equations \cite{murray or someone}, written in control-affine form as:\begin{align*}
    \dot {\b x} &= \b f_v(\b x) + \b g_v(\b x) \b u.
\end{align*}
for $v \in \{f, g\}$.

In the continuous domain, the dynamics are governed by the Euler Lagrange equations:
\begin{align*}
    \b M(\b q) \dot {\b v} = \b H(\b x) + \b B \b \tau + \b J_c(\b q)^\top \b \lambda
\end{align*}
where $\b M:\mathcal{Q} \to \R^{n\times n}$ is the symmetric positive definite mass-inertia matrix, $\b H:\mathcal{X}\to\R^n$ contains the gravitational and Coriolis forces, $\b B\in\R^n\times m$ is the selection matrix, $\b J_c:\mathcal{Q}\to\R^p$ is the Jacobian of the active holonomic constraints, and $\b\lambda\in\R^p$ are the ground reaction forces.

Associated with these respective domains are a set of transition surfaces, which define when one domain enters the next:
\begin{align*}
    \mathcal{S}_{f\to g} &\triangleq \{\b x \in \mathcal{D}_f~|~ p_z(\b q) = 0,~\dot p_z(\b x) < 0\}, \\ 
    \mathcal{S}_{g\to f} &\triangleq \{\b x \in \mathcal{D}_g~|~ \ell = 0,~\dot \ell < 0\}.
\end{align*}
The proposed method will design suitable controllers for discrete-time underactuated systems; therefore, we will next discuss how to model ARCHER via the discrete-time hop-to-hop dynamics. The hop-to-hop dynamics will be given by an endomorphism $\b F:\mathcal{S}_{f\to g} \to \mathcal{S}_{f\to g}$. Fixing a feedback controller $\b u = \b k(\b x)$ and let $\tau(\b x)$ return the time to impact for the closed loop system. That is, $\tau$  returns the time given a state until the robot's foot strikes the ground. With this, we can define the continuous time flow as:
\begin{align*}
    \b \varphi_1(\b x, \tau(\b x)) = \b x + \int_0^{\tau(\b x)} \b f(\b x(s)) + \b g_f(\b x(s))\b u(s) ds.
\end{align*}

As the robot impacts the ground, it undergoes a momentum transfer, written as:
\begin{align*}
        \b x^+ &= \b\Delta_{1,2}(\b x^-),
\end{align*}
whereby the robot enters the ground domain defined as . We can produce a mapping from $\b F_{1,2}: \mathcal{S}_1\to\mathcal{S}_2$ by considering the composition of flow and hybrid maps:
\begin{align*}
    \b x_2 = \b F_{1,2}(\b x_1) = \b \Delta_{1,2} \circ \b \varphi_{\tau(\b x)}(\b x_1)
\end{align*}
% We will next work to transform our system to a discrete time system. We model the dynamics of the hopping robot as a hybrid system \red{cite}, wherein the dynamics in the domain $\mathcal{D}_i$ are given by:

Parameterizing $\b u$ as being some discrete singal over the continuous domain, we can treat it as a discrete input.
Consider the composition of two of these to produce a cycle in the hybrid system graph: 
\begin{align*}
    \b x_{k+1} = \b F_{2,1} \circ \b F_{1,2}(\b x_k)
\end{align*}
Note that for the hopper, we could apply an input in the ground phase, but due to the fast nature of the system we choose not to. 
% Also, we assume that the impact time is not a function of orientation, which for for small angles is not a poor assumption, and was also made in \cite{nmpc_noel}.

Note that in doing this, we are electing to model the sytem via pre-impact to pre-impact event cycles.

                                Consider the output $\b y:\mathcal{Q} \to \R^m$ defined by:
\begin{align*}
        \b y(\b q) = \text{log}(q_d(\b z)^{-1} q) \\
        \dot{\b y}(\b\omega) = \b\omega - \b \omega_d
\end{align*}
